# Supplementary material for: Segmental Spatiotemporal CNNs for Fine-grained Action Segmentation
Source: arXiv:1602.02995 source file (2016-09-30)
Supplement: Supplementary file 1 [file appendix.tex]

\label{sec:appendix}
\section*{Sparsity}

\newcommand{\norm}[1]{\left\lVert#1\right\rVert}

In this section we show the gradients of the SSVM for various regularizers. See \cite{Bach?} for derivations of each norm.

The typical SSVM formulation given the data $X$ and ground truth labeling $y^*$, and weight matrix $w$ is
\begin{align}
J(w) = \norm{w}^2 + \frac{C}{N} \sum_{i=1}^N \max_{\hat{y}} \Delta(\hat{y}, y^*) + w^T (\Psi(X, \hat{y}) - \Psi(X, y^*))
\end{align}

If we precompute $\hat{y}$ we get:
\begin{align}
J(w; \hat{y}) = \norm{w}^2 + \frac{C}{N} \sum_{i=1}^N \Delta(\hat{y}, y^*) + w^T (\Psi(X, \hat{y}) - \Psi(X, y^*))
\end{align}

%For clarity let us abbreviate this as a function of the regularizer ($R(w)=\norm{w}^2$) and empirical risk ($L\sum_{i=1}^N \Delta(\hat{y}, y^*) + w^T (\Psi(X, \hat{y}) - \Psi(X, y^*))$.
%\begin{align}
%J(w) = \norm{w}^2 + \frac{C}{N} \sum_{i=1}^N \max_{\hat{y}} \Delta(\hat{y}, y^*) + w^T (\Psi(X, \hat{y}) - \Psi(X, y^*))
%\end{align}

For an arbitrary norm on the regularizer the gradient is:
\begin{align}
\nabla_w J(w; \hat{y}) = \nabla_w \norm{w}^2 + \frac{C}{N} \sum_{i=1}^N \Psi(X, \hat{y}) - \Psi(X, y^*)
\end{align}

If we use the L2 norm on the regularizer our gradient is 
\begin{align}
\nabla_w J(w; \hat{y}) = w + \frac{C}{N} \sum_{i=1}^N \Psi(X, \hat{y}) - \Psi(X, y^*)
\end{align}

If we use the L1 norm on the regularizer our gradient is the following. Note that we ignore the case where $w_{i,j}=0$.
\begin{align}
\nabla_w J(w; \hat{y}) = sign(w) + \frac{C}{N} \sum_{i=1}^N \Psi(X, \hat{y}) - \Psi(X, y^*)
\end{align}

If we use the L0 (nuclear) norm on the regularizer our gradient is the following where $U$ and $V^T$ are the matrices from the Singular Value Decomposition of $w$ such that $U,S,V^T = SVD(w)$. Note that we ignore the case where $w_{i,j}=0$.
\begin{align}
\nabla_w J(w; \hat{y}) = UV^T + \frac{C}{N} \sum_{i=1}^N \Psi(X, \hat{y}) - \Psi(X, y^*)
\end{align}

Finally, if we do not have a regularizer we simply have:
\begin{align}
\nabla_w J(w; \hat{y}) = \frac{C}{N} \sum_{i=1}^N \Psi(X, \hat{y}) - \Psi(X, y^*)
\end{align}

\section*{RNN objective}

\begin{align}
J(w) = \sum_{i=1}^N \sum_{t=1}^T \frac{1}{2} (y_t^* - a_t)^2
\end{align}

where we define the activation

\begin{align}
a_t = \text{sigmoid}(w_u^T X_t + \arg\max_{y_{t-1}} w_p^T \mathbf{1}[y_{t-1}, y] )
\end{align}

Note that this is a variation on the RNN where we assume the number of latent states is equal to the number of classes and we use a simple linear function on the data and pairwise terms as opposed to the common sigmoid and rectified linear unit functions.

For this case the gradients are as follows where $y_t=1$ for the correct class, $y_t=0$ for the incorrect class, and $e_t=y_t-a_t$:

\begin{align}
\nabla_{w_u} = \sum_{i=1}^N \sum_{t=1}^T e_t X_t^T
\end{align}

and 

\begin{align}
\nabla_{w_p} = \sum_{i=1}^N \sum_{t=1}^T e_t \mathbf{1}[y_{t-1}, y]^T  \text{[note: rewrite with } a_t?]
\end{align}

\section{Toy example}

\begin{figure}[tb]
  \includegraphics[width=\columnwidth]{imgs/toyexample/ToyExample_abcd.jpg}
  \caption{A toy example showing the effect of using semi-Markov model with and without a duration term. (a) Instances of action class 1 and action class 2. Action 2 is a phase shifted version of action 1 with an additional offset of 1.0. (b) test example with two consecutive instances of class 2. Segment scores for widths of 10 to 50 are depicted with dotted lines. A score greater than zero (incorrectly) corresponds to action 1 and less than zero (correctly) corresponds to action 2 (c) the ground truth action labels and the predicted labels using a linear classifier. Note that only the widest segment length correctly classifies the data for all timesteps (d) The predicted segment length at each timestep with and without a duration term.}
  \label{fig:ToyExample}
\end{figure}

We demonstrate the importance of using a submodular function with a toy example. In this example our data is generated by two sine waves with different offsets. See Figure~\ref{fig:ToyExample}a for the training data. The blue line (left) is a feature for an action of class $1$ and the red line (right) is a feature for an action of class $2$. Following the work of \cite{tao_miccai_2013} we use the mean function as the unary potential each segment. Let us start by modeling our energy as $E(X,Y) = \sum_{i=1}^M  w^T \phi(\mathbf{X}^s_i, \mathbf{Y}^s_i)$ where $\phi(\mathbf{X}^s_i, \mathbf{Y}^s_i)=\frac{1}{d_m}\sum_{t=1}^{d_m} X_{t}$ is a unary function, $M$ is the number of segments, and $d_m$ is the length of segment $m$.

Note that the mean function is not submodular. For submodularity to hold then $\phi(\mathbf{X}^s_{C}, \mathbf{Y}^s_C) \geq \phi(\mathbf{X}^s_{A}, \mathbf{Y}^s_A) + \phi(\mathbf{X}^s_{B}, \mathbf{Y}^s_B)$ for segments $A$, $B$, and $C$. If, for example, the mean values of $\phi$ for $A$, $B$, and $C$ respectively are 0.9, 1.1, and 1.0 then we see that our constraint does not hold: $1.0 \not\geq 0.9 + 1.1$. This model would break the segment into two parts.

Figure~\ref{fig:ToyExample}b depicts a test action sequence composed of two instances of class $B$ that are each 50 frames long. The dashed lines are the segment level scores for various segment lengths computed at each timestep. A score greater than 0 is labeled class $1$ and lower than 0 is labeled class $2$. The recognition accuracy is only 65.9\% due to the overlap between the two classes. Figure~\ref{fig:ToyExample}(c) shows the ground truth and inferred labels for the linear model at each timestep. 

Figure~\ref{fig:ToyExample}a (left) shows the inferred segment lengths at each timestep using the aforementioned model. Notice that the length is very short for most timesteps. We know from the training data that the sequences should never be that short; on average the actions are 50 frames long. We add a submodular duration term resulting in the energy 
\begin{align}
E(X,Y) = \sum_{i=1}^M { w_u^T \phi(\mathbf{X}^s_{i}, \mathbf{Y}^s_{i}) } + w_d^T \gamma(d_i)
\end{align}
where $\gamma(d) = [d, d^2]$. By adding this duration term we are able to correctly predict the sequence with 100\% accuracy. Figure~\ref{fig:ToyExample}a (right) shows the inferred segment lengths using the model with the duration term. As expected we see that the segment length increases until frame 50, after which point it labels the second instance of the action. In this example our energy becomes submodular when we use a duration term that biases the segment length to be at least 30.

%While the example depicted here uses a simple set of features and energy potentials, the same principles are applicable to more complex problems. 

% 
%\\
%\\
%\textbf{Potentials:}
The principles behind this result are applicable to a wide range of problems.
Common segment-level potential functions in the literature can be categorized into feature-based (e.g. mean, histogram, normalized-histogram), state-based (e.g. pairwise transition matrix), and duration-based (e.g. quadratic, Gaussian). We showed that the mean function is not submodular. In fact, any function that is normalized with respect to time will not be submodular. This includes normalized histograms, as used by \cite{tang_cvpr_2012,pirsiavash_cvpr_2014}, and others. The predicate-based potential that we proposed is also not submodular. Some potentials that are submodular include additive functions like the sum of features over a segment, un-normalized histograms, and duration potentials like a quadratic or Gaussian function. Pairwise state transitions are not submodular.
